# Supplementary material for: WeaverBird: Empowering Financial Decision-Making with Large Language Model, Knowledge Base, and Search Engine
Source: arXiv:2308.05361 source file (2024-04-07)
Supplement: Supplementary file 1 [file appendix-B.tex]

\section{System Details}\label{app:sys_details}
The system is based on the ChatGLM2-6B, we apply the LORA strategy to fine-tune the base model to adapt to the finance domain. The Lora layer details are as follows: the LORA rank is 16, the LORA alpha is 32, the dropout is 0.1, and other settings are default.

After retrieving relevant information from knowledge base and internet, we plug the information into the CONTEXT part of the following prompt template and feed it into the large language model. 
\begin{lstlisting}[caption={Prompt templates for LLM.},label={lst:prompt_template}]
English template:

Information:
{CONTEXT} 

Based on the given information, please provide a concise and professional response to the user's question. If a clear answer cannot be determined, respond with "Unable to answer the question based on the information provided" or "There is insufficient relevant information provided", without fabricating any part of the response. If there are multiple questions, answer all of them. You MUST respond in English! The question is: {QUESTION}.

Chinese template:
@\begin{CJK}{UTF8}{gbsn}已知信息：\end{CJK}@
{CONTEXT} 

@\begin{CJK}{UTF8}{gbsn}根据上述已知信息，简洁和专业地来回答用户的问题。如果无法从中得到答案，请说 “根据已知信息无法回答该问题” 或 “没有提供足够的相关信息”，不允许在答案中添加编造成分，如果提问中有多个问题，请一并回答，答案必须使用中文。 问题是：\end{CJK}@{QUESTION}.
\end{lstlisting}
