# Supplementary material for: WeaverBird: Empowering Financial Decision-Making with Large Language Model, Knowledge Base, and Search Engine
Source: arXiv:2308.05361 source file (2024-04-07)
Supplement: Supplementary file 2 [file appendix-G.tex]

\section{More Results}\label{app:results}
Now we present more examples of finance-related conversations of our WeaverBird system and other competing systems. 

\begin{lstlisting}[caption={About company dividend policy.},label={lst:div}]
@
\sethlcolor{humanpurple}  
\hl{
Query:
}
@  What is Microsoft's dividend policy and how does it compare to other companies in the technology sector?

@
\sethlcolor{aigreen}  
\hl{
WeaverBird:
}
@  Microsoft's dividend policy is to pay a quarterly dividend of $\$$0.68 per share. This means that for each share of Microsoft stock, its shareholders will receive $\$$0.68 every 3 months or 4 times per year. The company's dividend payments are typically made in the form of a quarterly dividend, which is a payment made by the company to its shareholders on a regular basis. When comparing Microsoft's dividend policy to other companies in the technology sector, it is important to consider the company's payout ratio, which is the percentage of its earnings that are paid out to shareholders as dividends. Microsoft's payout ratio is 66.1$\%$, which is relatively high compared to some other technology companies. For example, Apple, Microsoft's main competitor in the technology sector, pays a dividend of only 3.4$\%$ of its earnings out to shareholders. Google's dividend policy is similar to Microsoft's, but its payout ratio is lower at 52.5$\%$.

Overall, Microsoft's dividend policy is relatively high compared to other technology companies, and its shareholders can expect to receive regular dividends as the company continues to perform well.

// citations to information sources 
More details: 1. [Dividends Diversify], 2. [The Motley Fool], 3. [Seeking Alpha], 4. [Forbes], 5. [Barron's].
\end{lstlisting}

\begin{lstlisting}[caption={About business.},label={lst:bizbyd}]
@
\sethlcolor{humanpurple}  
\hl{
Query:
}
@ How many EVs has BYD sold in 2023? And what is the progress of BYD Europe expansion?

@
\sethlcolor{aigold}  
\hl{
ChatGPT:
}
@ As an AI language model, I cannot predict future events or sales figures. However, I can provide information about BYD's current progress in Europe. BYD has been expanding its presence in Europe through partnerships and investments in local companies. In 2021, the company announced a joint venture with Itochu to expand its electric bus business in Europe. BYD also plans to set up its first European battery factory in France and is working with Finnish company Visedo to develop electric drivetrains for marine vessels.

@
\sethlcolor{aired}  
\hl{
FinChat:
}
@ Based on the available data, the number of electric vehicles (EVs) sold by BYD in 2023 is not explicitly mentioned. However, we can analyze the revenue data to gain some insights. According to the "Automobiles and Related Products and Other Products Revenue" data source, for the semi-annual period ending on December 31, 2022, BYD generated CN@\begin{CJK}{UTF8}{gbsn}¥\end{CJK}@215.42B in revenue from the sale of automobiles and related products.

This represents a growth of 164.27%

However, we can look at the "Overseas Revenue" data source to gain some insights. For the semi-annual period ending on December 31, 2022, BYD generated CN58.07B in overseas revenue, representing a growth of 68.43%

This indicates that BYD's international operations, including its expansion into Europe, have been showing positive growth. In summary, while the exact number of EVs sold by BYD in 2023 is not provided, the strong revenue growth in the automobile segment suggests a robust performance in the EV market.

Additionally, the growth in overseas revenue indicates positive progress in BYD's expansion efforts, including in Europe.

@
\sethlcolor{aigreen}  
\hl{
WeaverBird:
}
@ Based on the information provided, BYD sold a total of 209,467 NEVs in the first half of 2023, which includes both pure battery electric and plug-in hybrid vehicles (PHEVs). Additionally, the automaker has set a goal of selling at least three million vehicles in 2023. As for the progress of BYD's Europe expansion, the company has sold a total of 1,255,637 NEVs in the first half of 2022... (long details omitted)

BYD is also expanding its global presence and has recently entered into a deal with European rental company SIXT... (long details omitted)

Overall, while the number of EVs sold by BYD in 2023 is not yet available, the company's progress in expanding its global presence and increasing its sales in Europe is promising.

More details: 1. [The Driven], 2. [Investor's Business Daily], 3. [CleanTechnica], 4. [InsideEVs], 5. [BYD].
\end{lstlisting}

\begin{lstlisting}[caption={About business.},label={lst:bizali}]
@
\sethlcolor{humanpurple}  
\hl{
Query:
}
@  Summarize Alibaba's last quarter with a focus on the cloud business. Include transcripts from CEO Daniel Zhang.

@
\sethlcolor{aigold}  
\hl{
ChatGPT:
}
@ Alibaba's last quarter was overall strong with a 34$\%$ increase in revenue year-over-year, totaling $\$$22.8 billion. The company's cloud computing business, Alibaba Cloud, continued to be a key driver of growth with a 59$\%$ increase in revenue year-over-year.

CEO Daniel Zhang commented on the success of the cloud business during the earnings call, stating, "Alibaba Cloud continued to deliver strong growth, driven by increased demand for public cloud and hybrid cloud offerings across all sectors and the growing adoption of our AI-powered data intelligence services." ... (long details omitted)

In addition to cloud computing, Alibaba's e-commerce business also saw growth, with a 30$\%$ increase in revenue year-over-year in their core commerce segment. The company also announced plans to invest $\$$28 billion over the next three years in their cloud infrastructure, as they continue to prioritize the growth of their cloud business.

@
\sethlcolor{aired}  
\hl{
FinChat:
}
@ Based on the available data, Alibaba's cloud business experienced a 2$\%$ year-over-year increase in revenue in the last quarter. This growth was partially influenced by adjustments in the revenue structure and changes in the market environment and customer composition.

The impact of a top customer switching to self-build infrastructure for its international business resulted in a 41%

Alibaba's Cloud Revenue for the most recent quarter was CN18.58B, representing a -2.05$\%$ growth compared to the previous quarter. Unfortunately, the provided data does not include specific details from CEO Daniel Zhang's transcript regarding Alibaba's cloud business in the last quarter.

@
\sethlcolor{aigreen}  
\hl{
WeaverBird:
}
@ Alibaba Group announced its June quarter 2022 results conference call on Tuesday, where CEO Daniel Zhang announced that he will be stepping down from his roles to focus on the company's cloud division. The company's cloud computing business saw significant growth, with revenues increasing 24$\%$ year over year. Eddie Wu was named the new CEO of Alibaba Group, following Zhang's departure.

More Details: 1. [TechCrunch] 2. [Reuters] 3. [Seeking Alpha] 4. [CNBC] 5. [The Motley Fool].
\end{lstlisting}

\begin{lstlisting}[caption={About business.},label={lst:biznvidia}]
@
\sethlcolor{humanpurple}  
\hl{
Query:
}
@ How will ChatGPT contribute to Nvidia's AI business in the short to medium term?

@
\sethlcolor{aigold}  
\hl{
ChatGPT:
}
@ It was recently reported that Nvidia has acquired ChatGPT, a Vietnamese AI startup that specializes in natural language processing. The acquisition is expected to contribute to Nvidia's AI business in the short to medium term in several ways:

1. Enhancing Nvidia's Conversational AI capabilities: ChatGPT's expertise in natural language processing will help to improve Nvidia's conversational AI capabilities, which are becoming increasingly important for virtual assistants and chatbots.

2. Strengthening Nvidia's AI platform: ChatGPT's technology and talent will likely be integrated into Nvidia's AI platform, which will help to strengthen the platform's capabilities and make it more competitive in the market.

3. Expanding Nvidia's customer base: ChatGPT has a diverse customer base, which includes large enterprises, startups, and research institutions. By acquiring ChatGPT, Nvidia will be able to expand its own customer base and target a wider range of industries.

Overall, the acquisition of ChatGPT is expected to help Nvidia to further establish itself as a leader in the AI space and to drive growth in its AI business in the short to medium term.

@
\sethlcolor{aired}  
\hl{
FinChat:
}
@ Based on the available data, there is no specific information regarding how ChatGPT will contribute to Nvidia's AI business in the short to medium term. The provided data sources do not mention any details about the impact of ChatGPT on Nvidia's AI business.

However, it is worth noting that Nvidia has expertise in AI supercomputers, algorithms, and data processing, which positions them well to leverage generative AI applications like ChatGPT. The transcript passages highlight the interest and potential of generative AI models like ChatGPT in improving productivity across various industries.

Nvidia's collaboration with OpenAI and their engagement with major cloud providers, consumer internet companies, enterprises, and startups further indicate their commitment to exploring and capitalizing on generative AI opportunities. While we don't have specific information about ChatGPT's contribution to Nvidia's AI business, it is reasonable to expect that Nvidia will continue to leverage their expertise and partnerships to drive growth in the AI space.

@
\sethlcolor{aigreen}  
\hl{
WeaverBird:
}
@  ChatGPT, as a generative AI model, will likely contribute to Nvidia's AI business in the short to medium term in several ways:

1. Increased Demand: As mentioned in the information provided, ChatGPT's parent company, OpenAI, has seen a massive increase in demand for its products, which could lead to a corresponding increase in Nvidia's revenue.

2. Positive Impact on Nvidia's Graphics Processing Units (GPUs): As the leading provider of graphics processing units, Nvidia can benefit from an increased demand for traditional AI and generative AI chatbots, which rely heavily on GPUs for processing power.

3. Expansion of Nvidia's Business: With the growing demand for ChatGPT and other AI models, Nvidia can expand its business and increase its market share in the AI industry.

4. New Revenue Streams: The development and deployment of ChatGPT can create new revenue streams for Nvidia, such as providing cloud-based services for AI developers and researchers.

In the short to medium term, ChatGPT can contribute to Nvidia's AI business by increasing demand... (long details omitted)

More Details: 1. [CNBC] 2. [Investor's Business Daily] 3. [NASDAQ] 4. [Yahoo Finance] 5. [Local Doc]. 
\end{lstlisting}

\begin{lstlisting}[caption={About individual opinions.},label={lst:opinion}]
@
\sethlcolor{humanpurple}  
\hl{
Query:
}
@ What does Tesla's Elon Musk think of BYD rivalry?

@
\sethlcolor{aigold}  
\hl{
ChatGPT:
}
@ Elon Musk, the CEO of Tesla, has not made any direct statements about BYD, a Chinese electric vehicle manufacturer that is often seen as a competitor to Tesla.

However, Musk has spoken about the broader competition in the electric vehicle market. In a 2019 interview with Automotive News, Musk acknowledged that there would be many electric vehicle competitors in the future, but he expressed confidence in Tesla's ability to succeed. He said, "I think it's going to be a very competitive market, like the car industry is. But I feel confident about where Tesla stands."

Musk has also praised China's progress in electric vehicle adoption and production. In 2019, he said, "I think China has some of the most impressive companies in the world. In particular, there are some really impressive companies in electric vehicles, like NIO and others. China is the largest market in the world for electric vehicles."

Overall, while Musk has not specifically addressed BYD, he has shown a general awareness of the competition in the electric vehicle market and expressed confidence in Tesla's ability to succeed.

@
\sethlcolor{aired}  
\hl{
FinChat:
}
@ Based on the provided data from Tesla's transcripts, Elon Musk acknowledges the competitiveness of Chinese car companies and the Chinese market. He mentions that the Chinese car companies are the most competitive in the world and that Tesla's China team is winning in China.

Musk also expresses respect for the car companies in China and believes that there is a high likelihood that a Chinese company could be the second most likely competitor to Tesla in the future. He further mentions that Tesla is able to attract the best talent in China.

Overall, Musk seems to have a positive outlook on the future and is excited about the competition in the market.

@
\sethlcolor{aigreen}  
\hl{
WeaverBird:
}
@ Tesla's Elon Musk now believes that BYD's vehicles are 'highly competitive' in China, according to a recent interview with him. In 2011, Musk laughed at the idea of China's BYD being a rival to Tesla, but it seems that his opinion has changed. The rival automakers pose the biggest challenge for Tesla in China, where the company is expected to be second in electric vehicles.

More Details: 1. [Fortune] 2. [Electrek] 3. [Yahoo Finance] 4. [Teslarati] 5. [InsideEVs]. 
\end{lstlisting}
