# Supplementary material for: WeaverBird: Empowering Financial Decision-Making with Large Language Model, Knowledge Base, and Search Engine
Source: arXiv:2308.05361 source file (2024-04-07)
Supplement: Supplementary file 3 [file appendix-C.tex]

\section{Implementation Details}\label{app:imple_details}

All models are implemented using the PyTorch framework \citep{paszke-17-pytorch}.

For the implementation of LangChain, we use the code from  the  public  GitHub  repository at {\small \url{https://github.com/imClumsyPanda/langchain-ChatGLM}}~\citep{langchainglm} without any License.

For the implementation of WebUI, we use the code from  the  public  GitHub  repository at {\small \url{https://github.com/THUDM/WebGLM}}~\citep{liu2023webglm} with Apache 2.0 License.

For the implementation of MAR@M and MAP@M, we used the code from  the  public  Github  repository at {\small \url{https://github.com/statisticianinstilettos/recmetrics}} without any license.
